# Supplementary material for: Sim and Real: Better Together
Source: arXiv:2110.00445 source file (2021-10-05)
Supplement: Supplementary file 1 [file appendix_old.tex]

\onecolumn
\section{Old Appendix} 
\label{app:Lemmas1And2}

% \input{lemma1_dotan_version}
% \input{distribution_RB}
% \input{TD_from_RB}
% \input{expectation_TD_Linear_FA}
% \input{k_environment}
\input{continuous_stationary}
\input{bounds_sim_real_critic}

\subsection{martingale difference - proofs for theorems}
Define the $\sigma$-algebra $\mathcal{F}_\tau \triangleq \{X_k: k \le \tau\}$ where $X_k$ is defined in Equation (\ref{eq:X_t}). Define
\[F_\tau^{\eta} \triangleq \mathbb{E}[\tilde r_{\tau, t} - \eta_\tau | \mathcal{F}_\tau]\]
\[M_{\tau+1, i}^\eta \triangleq (\tilde r_{\tau, t} - \eta_\tau) - F_\tau^{\eta}\]
\[F_\tau^{v} \triangleq \mathbb{E}[\delta_{\tau, t, i} \phi(\tilde s_{\tau, t}) | \mathcal{F}_\tau]\]
\[M_{\tau+1, i}^{v} \triangleq \delta_{\tau, t, i} \phi(\tilde s_{\tau, t}) - F_\tau^{v}\]
\[F_\tau^{\theta} \triangleq \mathbb{E}[\delta_{\tau, t, i} \nabla_\theta \log \pi_\theta (\tilde a_{\tau, t}| \tilde s_{\tau, t}) | \mathcal{F}_\tau]\]
\[M_{\tau+1, i}^{\theta} \triangleq \delta_{\tau, t, i} \nabla_\theta \log \pi_\theta (\tilde a_{\tau, t}| \tilde s_{\tau, t}) - F_\tau^{\theta}\]

%where the expectation is with respect to:
%\[\beta_i q_{j} P_j(s'| s, a) \cdot \pi_{\theta'_{\text{s2r-buffer}}} (a'| s') \cdot  \cdot \mathbb{P}(\mathcal{O}_j | X[\text{RB(I)}])\]


Using the above definitions, we can write the iterations:
\begin{equation}
\label{eq:eta_iteration2}
\eta_{\tau+1} = \eta_\tau + \alpha_\tau^{\eta} \left( F_\tau^{\eta} + M_{\tau+1, i}^\eta \right)
\end{equation}
\begin{equation}
\label{eq:v_iteration2}
    v_{\tau+1} = v_\tau + \alpha_\tau^{v} \left( F_\tau^{v} + M_{\tau+1, i}^v \right)
\end{equation}
\begin{equation}
\label{eq:theta_iteration}
    \theta_{\tau+1} = \theta_\tau + \alpha_\tau^{\theta} \left( F_\tau^{\theta} + M_{\tau+1, i}^\theta \right)
\end{equation}

We use Theorem 2.2 of \cite{borkar2000ode} to prove convergence of these iterates. Briefly, this theorem
states that given an iteration as in (\ref{eq:eta_iteration2}), (\ref{eq:v_iteration2}), and (\ref{eq:theta_iteration}) these iterations are bounded w.p.1 if

({\bf A1}) $F_\tau^{\eta}$, $F_\tau^{v}$ and $F_\tau^{\theta}$ are Lipschitz, the functions $F_\infty(\eta) = \lim_{\sigma \rightarrow \infty} F^{\eta} (\sigma \eta)/\sigma$, $F_\infty (v) = \lim_{\sigma \rightarrow \infty} F^{v} (\sigma v)/\sigma$ and $F_\infty(\theta) = \lim_{\sigma \rightarrow \infty} F^{\theta} (\sigma \theta)/\sigma$ are Lipschitz, and $F_\infty(\eta)$, $F_\infty(v)$ and $F_\infty(\theta)$ are asymptotically stable in the origin.

({\bf A2}) The sequences $M_{\tau+1, i}^{\eta}$, $M_{\tau+1, i}^{v}$ and $M_{\tau+1, i}^{\theta}$ are  martingale difference noises and for some $C_0^\eta$, $C_0^v$, $C_0^\theta$
\[\mathbb{E}\left[ (M_{\tau+1, i}^{\eta})^2 \middle| \mathcal{F}_\tau \right] \le C_0^\eta (1 + \| \eta_\tau \|^2)\]
\[\mathbb{E}\left[ (M_{\tau+1, i}^{v})^2 \middle| \mathcal{F}_\tau \right] \le C_0^v (1 + \| v_\tau \|^2)\]
\[\mathbb{E}\left[ (M_{\tau+1, i}^{\theta})^2 \middle| \mathcal{F}_\tau \right] \le C_0^\theta (1 + \| \theta_\tau \|^2)\]

For the average reward update, the ODE describing the asymptotic behavior of this recursion corresponds to
\[\dot \eta = - \eta + \mathbb{E}[r(s, a)] = F^\eta\]
$F^\eta$ is Lipschitz continuous in $\eta$. The function $F_\infty (\eta)$ exists and is simply $F_\infty (\eta) = -\eta$. The origin is an asymptotically stable equilibrium for the ODE
\[\dot \eta = F_\infty (\eta)\]
and the related Lyapunov function is given by $\eta^2/2$.

{\bf RB setting:}
Let's look at the chain:
\begin{align*}
    [s_\tau, \text{RB}_\tau] \overbrace{\rightarrow}^{\mathbb{P}(\tilde{\mathcal{O}}|\text{RB}_\tau)} \tilde{\mathcal{O}}_{\tau} \overbrace{\rightarrow}^{det} \theta_\tau \overbrace{\rightarrow}^{\pi} a_\tau \overbrace{\rightarrow}^{P_{\text{buf}}} [s_{\tau+1}, \text{RB}_{\tau+1}] \overbrace{\rightarrow}^{\mathbb{P}(\tilde{\mathcal{O}}|\text{RB}_{\tau+1})} \tilde{\mathcal{O}}_{\tau+1} 
    \overbrace{\rightarrow}^{det} \theta_{\tau+1} \overbrace{\rightarrow}^{\pi} a_{\tau+1}
\end{align*}
We can see that $\theta_{\tau}$ is based on an observation sampled from RB  $\tilde{\mathcal{O}}_{\tau} = \{\tilde{s}_{\tau, t, \cdot}, \tilde{a}_{\tau, t, \cdot}, r(\tilde{s}_{\tau, t, \cdot}, \tilde{a}_{\tau, t, \cdot}), \tilde{s}_{\tau, t+1, \cdot}\}$.

{\bf s2r setting}
Let's look at the chain:
\begin{align*}
    [s_\tau, \text{RB}_\tau, I_\tau, J_\tau] \overbrace{\rightarrow}^{\mathbb{P}(\tilde{\mathcal{O}}^J|\text{RB}_\tau (J_\tau))} \tilde{\mathcal{O}}^{J_{\tau}}_{\tau} \overbrace{\rightarrow}^{det} \theta_\tau \overbrace{\rightarrow}^{\pi} a_\tau  \overbrace{\rightarrow}^{P_{\text{s2r-buf}}} [s_{\tau+1}, \text{RB}_{\tau+1}, I_{\tau+1}, J_{\tau+1}]   \overbrace{\rightarrow}^{\mathbb{P}(\tilde{\mathcal{O}}^J |\text{RB}_{\tau+1}(J_{\tau+1}))} \tilde{\mathcal{O}}^{J_{\tau+1}}_{\tau+1} \\
    \overbrace{\rightarrow}^{det} \theta_{\tau+1} \overbrace{\rightarrow}^{\pi} a_{\tau+1}
\end{align*}
We can see that $\theta_{\tau}$ is based on the observation sampled from $\text{RB}_\tau(J_\tau)$ observation $\tilde{\mathcal{O}}^{J_\tau}_{\tau} = \{\tilde{s}_{\tau, t, J_\tau},\tilde{a}_{\tau, t, J_\tau}, r(\tilde{s}_{\tau, t, J_\tau}, \tilde{s}_{\tau, t, J_\tau}), \tilde{s}_{\tau, t+1, J_\tau} \}$.

Suppose we have a RB with $N$ samples, $RB = \{\mathcal{O}_1, \ldots, \mathcal{O}_N\}$. Without loss of generality, consider $\theta_1, \ldots, \theta_N$ as the actor parameters that are responsible for the transitions in  $\mathcal{O}_1, \ldots, \mathcal{O}_N$, respectively. 

\begin{remark}
The RB basically is a First-In-First-Out (FIFO) buffer. Without loss of generality, suppose the cells of this buffer are numbered from $1$ to $N$. The latest transition is pushed in cell $1$, the transition before that in cell $2$, etc. When a new transition arrives, the transition in cell $n$ moves to cell $n+1$ for $1\le n < N$, while the sample in $N$ is thrown away. We note that the sample in cell $n$ correspond to $\theta_{\tau-n}$.
\end{remark}

Let $P_{\theta_n}$ be a matrix with elements $P_{\theta_n}^{(ml)}$ in row $l$ and column $m$
\begin{equation*}
    P_{\theta_n}^{(ml)} \triangleq P(s'=m| s=l) = \sum_{a \in \mathcal{A}} P(s'|s,a) \pi_{\theta_{n}} (a|s).
\end{equation*}
We denote by $\rho_n$ the  distribution of states in position $n$ in the RB, which satisfies
\begin{align*}
    \rho_{n+1}^\top &= \rho_{n}^\top P_{\theta_{n}}\\
    \Rightarrow \rho_{n+2}^\top &= \rho_{n}^\top P_{\theta_{n}} P_{\theta_{n+1}}\\
    \ldots \Rightarrow \rho_{n+n'}^\top &= \rho_{n}^\top \prod_{t=n}^{n+n'-1}  P_{\theta_{t}}
\end{align*}

Let $\bold{R}_{\theta_n} \in \mathbb{R}^{|\mathcal{S}| \times |\mathcal{S}|}$ be a diagonal matrix with elements of the vector $\bold{r}_{\theta_n}$ where $\bold{r}_{\theta_n}$ is a column vector $\big( \sum_a \pi_{\theta_n}(a|s) r(s_1, a), \ldots \sum_a \pi_{\theta_n}(a|s) r(s_{|\mathcal{S}|}, a) \big)^\top$. We denote by $\upsilon_n$ the distribution of reward for each state and action in position $n$ in the RB, which satisfies
\begin{align*}
 \upsilon_{n+1}^\top &= \rho_{n}^\top \bold{R}_{\theta_{n}} \\
    \upsilon_{n+2}^\top &= \rho_{n+1}^\top \bold{R}_{\theta_{n+1}} = \rho_{n}^\top P_{\theta_{n}} \bold{R}_{\theta_{n+1}}\\
    \upsilon_{n+3}^\top &= \rho_{n+2}^\top \bold{R}_{\theta_{n+3}} = \rho_{n}^\top P_{\theta_{n}} P_{\theta_{n+1}} \bold{R}_{\theta_{n+2}}\\
    \ldots \Rightarrow \upsilon_{n+n'}^\top &= \rho_{n}^\top \prod_{t=n}^{n+n'-2}  P_{\theta_{t}} \cdot \bold{R}_{\theta_{n+n'-1}}
\end{align*}

Recall the our TD-error update is defined as:
\[\delta(\tilde{\mathcal{O}}) = \tilde r - \eta_\theta + \phi(\tilde s')^\top v -  \phi(\tilde s)^\top v.\]
Let $\tilde{\mathcal{O}}^z = \{\tilde s^z, \tilde a^z, \tilde r^z, \tilde {s'}^{z}\}$. In the critic update we use an empirical mean over several sampled observations, denoted as $\{\tilde{\mathcal{O}}^z\}_{z=1}^{N_{\text{samples}}}$. Then the critic update is defined as
\[v' = v + \alpha^v \frac{1}{N_{\text{samples}}} \sum_{z}\delta(\tilde{\mathcal{O}}^z) \phi (\tilde s^z)\]

Consider $N_{\text{samples}} = 1$. For critic updates, consider the following ODE:
\begin{align}
\label{eq:ode_v}
    \nonumber \dot v & = \mathbb{E}_{\tilde{\mathcal{O}} \sim \text{RB}} \left[\delta(\tilde{\mathcal{O}}) \phi (\tilde s) \right]\\
    \nonumber & = \mathbb{E}_{\tilde{\mathcal{O}} \sim \text{RB}} \left[(\tilde r - \eta_\theta + \phi(\tilde s')^\top v -  \phi(\tilde s)^\top v) \phi (\tilde s) \right] \\
    \nonumber & = \mathbb{E}_{\theta_n} \left[ \mathbb{E}_{\rho_n} \left[(\tilde r - \eta_\theta + \phi(\tilde s')^\top v -  \phi(\tilde s)^\top v) \phi (\tilde s) \middle| \theta_n \right] \right] \\
    \nonumber & = \sum_{n=1}^N P(\theta_n) \cdot  \mathbb{E}_{\rho_n} \left[(\tilde r - \eta_\theta + \phi(\tilde s')^\top v -  \phi(\tilde s)^\top v) \phi (\tilde s) \middle| \theta_n \right] \\
    & \overbrace{=}^{???} \frac{1}{N}\sum_{n=1}^N  \sum_{\tilde {s}} \rho_n (\tilde {s}) \left[(\tilde r - \eta_\theta + \phi(\tilde s')^\top v -  \phi(\tilde s)^\top v) \phi (\tilde s) \middle| \theta_n \right] = F^v
    % [ \big(r(s,a) - J(\theta) \\
    %& + v^\top \sum_{s' \in \mathcal{S}} P_i (s' | s, a) \phi(s') - v^\top \phi(s) \big) \phi(s) = F^v
\end{align}
where $\mathbb{E}_{\tilde{\mathcal{O}} \sim \text{RB}}$ denotes expectation w.r.t sampling from a RB. Since we sample from the RB i.i.d, then $P(\theta_n) = \frac{1}{N}$. 




Let $\rho_0$ the initial state distribution in RB before the first transition enters, at time $\tau-N$. \sd{rephrase}. Then, \\
\noindent \textbf{1.} The vector $\bold{s}$ is
\begin{align*}
    \bold{s}^\top & = \frac{1}{N} \sum_{n=1}^N \rho_{n}^\top \\
    & = \frac{1}{N} \big( \rho_{1}^\top + \rho_{2}^\top + \ldots + \rho_{N}^\top \big)   \\
    & = \frac{1}{N} \big( \rho_{0}^\top P_{\theta_0} + \rho_{0}^\top P_{\theta_0} P_{\theta_1} + \ldots + \rho_{0}^\top P_{\theta_0} P_{\theta_1} \cdots P_{\theta_{N-1}}  \big)   \\
    & = \rho_{0}^\top \frac{1}{N}  \sum_{n=1}^N 
    \prod_{t=0}^{n-1} P_{\theta_t}.
\end{align*}
\noindent \textbf{2.} The vector $\bold{s'}$ is
\begin{equation}
    \bold{s}'^\top = \frac{1}{N} \sum_{n=1}^N \rho_{0}^\top
    \prod_{t=0}^{n} P_{\theta_t}.
\end{equation}
Let $\bold{S}$ and $\bold{S'}$ be diagonal matrices with elements of the vectors $\bold{s}$ and $\bold{s'}$, respectively, along their diagonal. 
\begin{remark}
Notice that both $\bold{s}$ and $\bold{s'}$ are composed from a sum of $N$ vectors, divided by $N$. Each of the element in the summation is composed from an inner product of a stochastic vector $\rho_{0}$ and a product of stochastic matrices $P_{\theta_n}$. Therefore,  $\bold{s}$ and $\bold{s'}$ are stochastic vectors. 
\end{remark}

Both $\bold{S}$ and $\bold{S'}$ are row-stochastic matrices since they are composed of a sum of $N$ matrices, each of which is by itself product of row stochasic matrices $P_{\theta_n}$
\begin{remark}
If $N=1$, then we receive the online case: $\bold{s}^\top = \rho_{0}^\top
    P_{\theta_0} = \rho_{0}^\top
    \sum_{a \in \mathcal{A}} P(s'|s,a) \pi_{\theta_{0}} (a|s) = \rho_{0}^\top P(s'|s)$.
\end{remark}



%Let $\bold{D} \in \mathbb{R}^{|\mathcal{S}| \times |\mathcal{S}|}$ be a diagonal matrix with elements of the vector $\bold{s}$ along its diagonal. 

%\sd{Or: 
%Let $\mu_{\bold{S}}$ be the stationary distribution of the matrix $\bold{S}$, satisfying:
%\[\mu_{\bold{S}}^\top = \mu_{\bold{S}}^\top \bold{S}\]
%Let $\bold{D} \in \mathbb{R}^{|\mathcal{S}| \times |\mathcal{S}|}$ be a diagonal matrix with elements of the vector $\mu_{\bold{s}}$ along its diagonal. 
%}

%The transition of the consecutive states $(s, s')$ where $s, s'\in \mathcal{S}$ in the RB are expressed with the matrix $\bold{S} \triangleq \bold{s} \bold{s}'^\top$ where the row correspond to $s$ and the column correspond to $s'$.

We now denote a new vector $\bold{r}$ 
\begin{align*}
    \bold{r}^\top & = \frac{1}{N} \sum_{n=1}^N \upsilon_{n}^\top \\
    & = \frac{1}{N} \big( \upsilon_{1}^\top + \upsilon_{2}^\top + \ldots + \upsilon_{N}^\top \big)   \\
    & = \frac{1}{N} \big( \rho_{0}^\top \bold{R}_{\theta_0} + \rho_{0}^\top P_{\theta_0} \bold{R}_{\theta_1} + \ldots + \rho_{0}^\top P_{\theta_0} P_{\theta_1} \cdots P_{\theta_{N-2}} \cdot \bold{R}_{\theta_{N-1}} \big)   \\
    & = \rho_{0}^\top \frac{1}{N}  \sum_{n=1}^N 
    \Big( \prod_{t=0}^{n-2} P_{\theta_t} \Big) \cdot \bold{R}_{\theta_{n-1}}. 
\end{align*}

\begin{remark}
If $N=1$, then we receive the online case: $\bold{r}^\top = \rho_{0}^\top R_{\theta_0}$.
\end{remark}

In vector-matrix notation, (\ref{eq:ode_v}) is analogous to
%\[ \dot v = \boldsymbol{\Phi}^\top {\bf D} \big( {\bf r} -\eta_\theta {\bf e} +  \bold{S} \boldsymbol{\Phi} v  - \boldsymbol{\Phi} v \big),\]
\begin{align*}
    \dot v & = \boldsymbol{\Phi}^\top {\bf r} - \eta_{\theta} \boldsymbol{\Phi}^\top {\bf e}  + \boldsymbol{\Phi}^\top \bold{S'} \boldsymbol{\Phi} v -  \boldsymbol{\Phi}^\top {\bf S}   \boldsymbol{\Phi} v. \\
    & = \boldsymbol{\Phi}^\top \Big( {\bf r} - \eta_{\theta} {\bf e} + \bold{S'} \boldsymbol{\Phi} v - {\bf S}   \boldsymbol{\Phi} v \Big). \\
    & = \boldsymbol{\Phi}^\top \Big( {\bf r} - \eta_{\theta} {\bf e} + \big( \bold{S'} - {\bf S} \big)  \boldsymbol{\Phi} v \Big).
\end{align*}

%where ${\bf r}$ being the column vector $\big( \sum_a \pi(a|s) r(s_1, a), \ldots \sum_a \pi(a|s) r(s_{|\mathcal{S}|}, a) \big)^\top$ \sd{check, maybe needs to be redefined}



%Let ${\bf R}$ be a diagonal matrix with elements of $\bold{r}$ along its diagonal. 
\sd{continue from here}
$F^v$ is Lipschitz continuous in $v$ and $F_\infty (v)$ exists and equals 
%\[F_\infty (v) = \boldsymbol{\Phi}^\top {\bf D} \big( \bold{S}  - {\bf I} \big) \boldsymbol{\Phi} v\]
\[F_\infty (v) = \boldsymbol{\Phi}^\top \big( \bold{S'} - {\bf S} \big)  \boldsymbol{\Phi} v\]
%where ${\bf I}$ is the identity matrix. 
Consider the system
\begin{equation}
\label{eq:ode_v_infty}
    \dot v =F_\infty (v)
\end{equation}
Note that the matrix $\bold{S}$ has a simple eigenvalue of one and its remaining eigenvalues have real parts that are less than one. Thus $(\bold{S} - {\bf I})$ will have one eigenvalue of zero and other eigenvalues with negative real parts. Also, corresponding to the eigenvalue zero, the matrix $(\bold{S} - {\bf I})$ has a left
eigenvector $\mu^{\theta \top}$ and a right eigenvector ${\bf e} = (1 \ldots 1)^\top$ 
(the $|\mathcal{S}|$-dimensional unit vector), respectively. Thus, in principle, the set of asymptotically stable fixed points of (\ref{eq:ode_v_infty}) would correspond to the set $\{\alpha v | \boldsymbol{\Phi} v = {\bf e} \text{ and } \alpha \in \mathbb{R}, \alpha \neq 0\} \cup \{v = 0\}$.  Note that the two sets in the union (above) are disjoint. Now by the second part of Assumption \ref{ass:independent_features}, $\boldsymbol{\Phi} v \neq {\bf e}$, for every $v \in \mathbb{R}^d$. Thus the only asymptotically stable equilibrium for (\ref{eq:ode_v_infty}) is the origin.

Now, from average reward, TD-error, and critic updates define $N^1(t), M^1(t)$, $t \ge 0$, according to
\[N^1(t) = r_t - \mathbb{E}[r_t | \mathcal{F}_1(t)]\]
\[M^1(t) = \delta_{t;i}\phi(\tilde s_t ; i) - \mathbb{E}[\delta_{t;i}\phi(\tilde s_t ; i) | \mathcal{F}_1(t)]\]
respectively, where $\mathcal{F}_1(t) = \sigma ({\bf v}_r, \hat J_r, N^1(r), M^1(r), r \le t)$.  It is easy to see that 
\[\mathbb{E}[ \|N^1(t+1)\|^2 | \mathcal{F}_1(t)] \le C_1 (1 + \| \hat J_t\|^2 + \| {\bf v}_t\|^2 ), t \ge 0\]
\[\mathbb{E}[ \|M^1(t+1)\|^2 | \mathcal{F}_1(t)] \le C_2 (1 + \| \hat J_t\|^2 + \| {\bf v}_t\|^2 ), t \ge 0\]
for some $C_1, C_2 < \infty$. In fact, quantities $N^1(t)$ can be directly seen to be uniformly bounded almost surely. Thus Assumptions (A1) and (A2) of \cite{borkar2000ode} can be seen to be satisfied in the case
of the average reward, the TD-error, and the critic updates. From Theorem 2.1 of \cite{borkar2000ode}, average reward, TD-error, and critic iterates are uniformly
bounded with probability one. Now note that XXX has $J(\pi)$ defined as in XXX as its unique globally asymptotically stable equilibrium with $V_2(\eta) = (\eta - J(\pi))^2 $ serving as the associated Lyapunov function.

Next, suppose that ${\bf v} = {\bf v}^\pi$ is a solution to the system
\[\boldsymbol{\Phi}' {\bf D} \boldsymbol{\Phi} {\bf v} = \boldsymbol{\Phi}' {\bf D} T(\boldsymbol{\Phi} {\bf v})\]
We show that ${\bf v}^\pi$ is the unique globally asymptotically stable equilibrium of the ODE XXXX with the function $W(\cdot)$ defined by
\[W({\bf v}) = \frac{1}{2} \Big(\boldsymbol{\Phi}^\top {\bf D} \big( T(\boldsymbol{\Phi} {\bf v})  - \boldsymbol{\Phi} {\bf v} \big) \Big)^\top \Big(\boldsymbol{\Phi}^\top {\bf D} \big( T(\boldsymbol{\Phi} {\bf v})  - \boldsymbol{\Phi} {\bf v} \big) \Big)\]
serving as an associated strict Lyapunov function. Thus note that
\[\nabla W({\bf v}) = \boldsymbol{\Phi}^\top ({\bf P}^\pi - {\bf I})^\top {\bf D} \boldsymbol{\Phi} \boldsymbol{\Phi}^\top {\bf D} \big( T(\boldsymbol{\Phi} {\bf v})  - \boldsymbol{\Phi} {\bf v} \big)\]
Hence:
{\small
\begin{align*}
    & \frac{dW({\bf v})}{dt} = \nabla W({\bf v})^\top \dot {\bf v} \\
    & = \big( T(\boldsymbol{\Phi} {\bf v})  - \boldsymbol{\Phi} {\bf v} \big)^\top  {\bf D} \boldsymbol{\Phi} \boldsymbol{\Phi}^\top {\bf D} ({\bf P}^\pi - {\bf I}) \boldsymbol{\Phi} \boldsymbol{\Phi}^\top {\bf D} \big( T(\boldsymbol{\Phi} {\bf v}^\pi)  - \boldsymbol{\Phi} {\bf v} \big)
\end{align*}
}
According to assumption XXXX, for any ${\bf b} \in \mathbb{R}^d$, $\boldsymbol{\Phi} {\bf b}$ is a non-constant vector (i.e., one that is not of the form $\alpha {\bf e}$ for $\alpha \neq 0$). Thus ${\bf b}^\top \boldsymbol{\Phi}^\top {\bf D}({\bf P}^\pi - {\bf I}) \boldsymbol{\Phi} {\bf b} < 0$, $\forall {\bf b} \neq {\bf 0}$, i.e.,
the matrix $\boldsymbol{\Phi}^\top {\bf D}({\bf P}^\pi - {\bf I}) \boldsymbol{\Phi}$ is negative definite. Now any $\hat {\bf v} = {\bf v}^\pi + \alpha {\bf v}$, with $\alpha \in \mathbb{R}, \alpha \neq 0$ and ${\bf v}$ such that $\boldsymbol{\Phi} {\bf v} = {\bf e}$  will also be a solution to the linear system of equations XXX. However, again by Assumption (A3),  $\boldsymbol{\Phi} {\bf v} \neq {\bf e}$ for any ${\bf v} \in \mathbb{R}^d$. Thus any $\hat {\bf v}$ as above will not be a solution and the only solution is ${\bf v} = {\bf v}^\pi$ which is therefore unique. Thus,
\[\frac{dW({\bf v})}{dt} < 0 \text{ on the set } \{{\bf v} \in \mathbb{R}^d| {\bf v} \neq {\bf v}^\pi\}\]
and 
\[\frac{dW({\bf v})}{dt} = 0 \text{ on the set } \{{\bf v} = {\bf v}^\pi\}\]
Thus for XXX, ${\bf v}^\pi$ is the unique globally asymptotically stable equilibrium. The assumptions (A1)-(A2) of \cite{borkar2000ode} are now verified and the claim follows from Theorem 2.2, pp. 450 of \cite{borkar2000ode}.


and we have
\[F_\infty (v) = \lim_{\sigma \rightarrow \infty} F^{v} (\sigma v)/v = \mathbb{E}[(\phi' - \phi)\phi^\top]v\]
Thus, it is easy to show, using Assumption \ref{ass:independent_features}, that the ODE $\dot v = F_\infty^v  $ has a unique global asymptotically stable point at the origin and ({\bf A1}) is valid. For ({\bf A2}) we have
\begin{align*}
    \mathbb{E}\left[ \|M_{\tau+1, i}^{v}\|^2 \middle| \mathcal{F}_\tau \right]  & \le \mathbb{E}\left[ \|\delta_{\tau, t, i} \phi(\tilde s_{\tau, t})\|^2 \middle| \mathcal{F}_\tau \right] \\
    & \le 2 \| B_r + B_\eta + 4 B_\phi^2 v_\tau \|^2\\
    & \triangleq C_0^v (1 + \| v_\tau \|^2)
\end{align*}


where the first inequality results from the inequality $\mathbb{E}[(x - \mathbb{E}[x])^2] \le \mathbb{E}[x^2]$,
and the second inequality results from the uniform boundedness of the involved variables. We note that the related ODE for this iteration is given by $\dot v = F^v  $, and the related Lyapunov function is given by $\mathbb{E}[\delta^2]$. 

\subsection{Critic convergence for $K$ environments}
Let us look at the Markov chain $\{s_0, s_1, \ldots ....\}$. Let $d_t(s)$ be the Markov chain distribution of states at time $t$, that is
\[d_t^\top = d_0^\top \prod_{t'=1}^t P_{\theta_t'}\]
for some initial state distribution $d_0$. 
In our process, we observe state $s_t$, choose environment $i$ with probability $q_i$, sample next state according to $P_i$ and store the transition $\mathcal{O}_t = \{s_t, a_t, r_t, s_{t+1}\}$ in $\text{RB}(i)$. 

Let $P^i_{\theta_n}$ be a matrix with elements $P_{\theta_n}^{i, (ml)}$ in row $l$ and column $m$
\begin{equation*}
    P_{\theta_n}^{i, (ml)} \triangleq P_i(s'=m| s=l) = \sum_{a \in \mathcal{A}} P_i(s'|s,a) \pi_{\theta_{n}} (a|s).
\end{equation*}
where $P_i(\cdot|\cdot, \cdot)$ is the state transition probability of environment $M_i$ given an action. 

Let us fix time $\tau$. We denote the time index of entering a transition into $\text{RB}(i)$ as  $t_n^i \in \{0, \ldots, \tau-1\}$ for all $i \in \{1, \ldots, K \}$, and for all $n \in \{ 1, \ldots \}$
\begin{remark}
Note that each time step that a transition enters some $\text{RB}(\cdot)$ is unique, meaning: $t_n^i \neq t_n^j$ for all $n$ and for $i \neq j$. Moreover, $t_n^i < t_{n+1}^i$ for all $i$ and all $n$. 
\end{remark}

%Let $\mathcal{O}_{t_n^i} = \{ s_{t_n^i}, a_{t_n^i}, r_{t_n^i}, s_{t_n^i+1}\}$ where $s_{t_n^i+1} \sim P_i(\cdot | s_{t_n^i})$.


We denote by $\rho_n^i$ the distribution of states in position $n$ in $\text{RB}(i)$, which satisfies
\begin{align*}
    \rho_{0}^{i \top} &= d_{t_0^i - 1}^{\top}\\
    \rho_{1}^{i \top} &= d_{t_1^i - 1}^{\top} \\
    \ldots \Rightarrow \rho_{n}^{i \top} &= d_{t_n^i - 1}^{\top}
\end{align*}
Let us look at:
\begin{align*}
    \mathbb{E}_{\text{RB}}[\delta(\tilde{\mathcal{O}} \phi(\tilde s)] & = \ldots = \Phi^{\top} \left( \sum_{j=1}^K \beta_j \frac{1}{N} \sum_{n=1}^N S^j_{\theta_n} \left( \sum_{i=1}^K q_i P^i_{\theta_n} - I \right) \right) \Phi v + \phi^T \left(  \sum_{j=1}^K \beta_j \frac{1}{N} \sum_{n=1}^N S^j_{\theta_n} \right) (r - \eta)
\end{align*}
where
\begin{align*}
     S^j_{\theta_n} & = \text{diag} (\rho_{n}^{j \top}) = \text{diag} \left( d_{t_n^i - 1}^{\top} \right) = \text{diag} \left(d_0^\top \prod_{t'=1}^{t_n^i - 1} P_{\theta_t'} \right)
\end{align*}

\subsection{Original lemmas}
For the actor updates Procedure \ref{alg:linear_actor_critic}, we use a projection operator $\Gamma: \mathbb{R}^d \rightarrow \mathbb{R}^d$ that projects any $x \in \mathbb{R}^d$ to a compact set $C = \{x | q_i(x) \leq 0, i=1, \ldots, m \} \subset \mathbb{R}^d$ where $q_i(\cdot)$ are real-valued, continuously differentiable functions on $\mathbb{R}^d$
that represent the constraints specifying the (above) compact region. The projection method is an often used technique to ensure boundedness of iterates in stochastic approximation algorithms, see \citet{bhatnagar2009natural} for further details.

Let $P(s'|s,a)$ be the transition probability of MDP $M$ such as:
\[P(s'|s,a) = \sum_{i=1}^K q_i P_i(s'|s,a), \ \forall s,s' \in \mathcal{S}, a \in \mathcal{A},\]
where $q_i$ satisfy $q_i \ge 0$ and $\sum_{i=1}^K q_i = 1$. We denote by $\boldsymbol{\beta}$ the vector with entries $q_i$. Let $\mu_\theta$ be the stationary distribution for MDP $M$, induced by the policy $\pi_\theta$. The gradient of the critic loss is then: 
\begin{align*}
    \nabla_{{\bf w}} \mathcal{E}^{\pi_\theta}_{\text{s2r}} ({\bf w}) & = - \mathbb{E}_{s \sim \mu_\theta, a \sim \pi_{\theta}} \big[ \big( Q^{\pi_\theta} (s,a) - \hat{Q}^{\pi_\theta}_{{\bf w}}(s,a) \big) \\
    & \nabla_{{\bf w}} \hat{Q}^{\pi_\theta}_{{\bf w}}(s,a) \big]
\end{align*}
We estimate this gradient by a single transition sample from one of the replay buffers RB $i; i \in (1, \ldots K)$. We define two new  functions, denoted  by $Q^{\pi_\theta} (s,a; i)$ and $V^{\pi_\theta} (s; i)$, which use the transition probability matrix ${\bf P}_i$ of MDP $M_i$: 
\begin{equation}
\label{eq:Q_i2}
    Q^{\pi_\theta} (s,a; i) \triangleq r(s,a) - \eta(\boldsymbol{\theta}) + \sum_{s'} {\bf P}_i(s'|s,a) V^{\pi_\theta} (s')
\end{equation}
\begin{equation}
\label{eq:V_i2}
    V^{\pi_\theta} (s; i) \triangleq \sum_{a} \pi_\theta(a|s) Q^{\pi_\theta} (s,a; i)
\end{equation}
Using $ Q^{\pi_\theta} (s,a; i)$ we estimate the gradient of the critic loss by $\hat \nabla_{{\bf w}} \mathcal{E}^{\pi_\theta}_{\text{s2r}} ({\bf w})$:
\begin{align}
\label{eq:critic_loss_gradient}
    \hat \nabla_{{\bf w}} \mathcal{E}^{\pi_\theta}_{\text{s2r}} ({\bf w}) & =  - \big( Q^{\pi_\theta} (s,a; i) -  \hat{Q}^{\pi_\theta}_{{\bf w}}(s,a) \big) \nabla_{{\bf w}} \hat{Q}^{\pi_\theta}_{{\bf w}}(s,a).
\end{align}

We begin with the first lemma: 

\begin{lemma}
\label{lemma:Q_expec3}
\[(a) \mathbb{E}_{i \sim \boldsymbol{\beta}} [Q^{\pi_\theta} (s,a; i) \psi(s,a)] = Q^{\pi_\theta} (s,a) \psi(s,a)\]
\[(b) \mathbb{E}_{i \sim \boldsymbol{\beta}} [\hat Q^{\pi_\theta}_{\bf w} (s,a) \psi(s,a)] = \hat Q^{\pi_\theta}_{\bf w} (s,a) \psi(s,a)\]

\end{lemma}
The proof is in the appendix. 

We next show that $\hat \nabla_{{\bf w}} \mathcal{E}^{\pi_\theta}_{\text{s2r}} ({\bf w})$ is an unbiased estimate for the real gradient $\nabla_{{\bf w}} \mathcal{E}^{\pi_\theta}_{\text{s2r}} ({\bf w})$.
\begin{lemma}
\label{lemma:unbiased_critic_gradient2}
\[ \mathbb{E} \big[ \hat \nabla_{{\bf w}} \mathcal{E}^{\pi_\theta}_{\text{s2r}} ({\bf w})\big] = \nabla_{{\bf w}} \mathcal{E}^{\pi_\theta}_{\text{s2r}} ({\bf w}) \]
\end{lemma}

Let $\tilde {\mathcal{O}}_{t;i} = \{\tilde s_{t}, \tilde a_{t}, \tilde s'_{t}, \tilde r_{t}\}$ be a transition sampled at time $t$ from  $RB_t(i)$. Note that $\tilde o_{t;i}$ is a transition sampled from a RB, and it is {\bf not} necessarily the last transition in the Markov chain $\mathcal{O}_{t} = \{s_{t}, a_{t}, s_{t+1}, r_{t}\}$.

The temporal difference (TD) error $\delta_{t; i}$ is a random quantity,  based on a single transition from $RB_t(i)$, and is defined according to:
\begin{equation}
\label{eq:delta_def2}
    \delta_{t; i} \triangleq \tilde r_{t} - \eta_{t} + \hat{V} \big( \tilde s'_{t} \big) - \hat{V} \big( \tilde s_t \big)
\end{equation}

where $\hat{V} \big( \tilde s_{t} \big)$ and $\hat{V} \big( \tilde s'_{t} \big)$
are unbiased estimates of the value function in states $ \tilde s_{t}$ and $\tilde s'_{t}$. Likewise, $\eta_{t}$ is an unbiased estimates of the average reward from MDP $M$. Thus, in particular, these estimates satisfy:

\[\mathbb{E}[\hat{V} \big( \tilde s_{t}\big) | \tilde s_{t}, \pi_\theta] = V^{\pi_\theta}  \big( \tilde s_{t} \big)\]
\[\mathbb{E} [\eta_{t}  | \tilde s_{t}, \pi_\theta] = \eta_{\boldsymbol\theta} \]
Respectively, for any $t > 0$. We assume here that actions are chosen according to policy $\pi_{\theta}$. 

Next, we show that even if we use a single transition $\tilde o_{t;i}$ from RB i to estimate the TD error $\delta_{t; i}$, the conditional expectation of $\delta_{t; i}$ equals the advantage function. 

\begin{lemma}
\label{lemma:unbiased_delta}
\begin{align*}
    \mathbb{E}[\delta_{t; i} | \tilde s_{t}, \tilde a_{t}, \pi_\theta] = A^{\pi_\theta} (\tilde s_{t} , \tilde a_{t})
\end{align*}
\end{lemma}
The proof is based on Lemma 3 in \cite{bhatnagar2009natural}, adapted to our scheme, and it appears in the appendix. 


By setting the baseline $b(s)$ equal to the value functions $V^{\pi_\theta} (s)$
The gradient of $\eta_\theta$ can be written as
\[\nabla \eta_\theta = \mathbb{E}_{s \sim \mu_\theta, a \sim \pi_\theta} [\psi(s,a) A^{\pi_\theta} (s,a)] \]
From Lemma \ref{lemma:unbiased_delta}, $\delta_{t; i}$ is an unbiased estimate of the advantage function $A^{\pi_\theta} (\tilde s_{t}, \tilde a_{t})$. Thus, $\hat \nabla \eta_\theta = \psi(\tilde s_{t}, \tilde a_{t}) \delta_{t; i} $ is an unbiased estimate of $\nabla \eta_\theta$. However, calculating  $\delta_{t; i}$ requires having estimates, $\eta_t, \hat V(\tilde s_t)$ and $\hat V(\tilde s'_t)$, of the average reward and the value function. While an average reward estimate is simple enough to obtain given the single-stage reward function, the same is not necessarily true for the value function. We use function approximation for the value functions as well. Suppose $\phi(s)$ is a $d$-dimensional feature vector for state $s$. One may then approximate $V^{\pi_\theta}(s)$ with ${\bf v}^\top \phi(s)$, where ${\bf v}$ is a
$d$-dimensional weight vector which can be tuned (for a fixed policy $\pi$) using a TD algorithm. In our algorithms, we then use
\begin{align}
\label{eq:delta_linear}
    \delta_{t; i} = \tilde r_{t} - \eta_t + {\bf v}_t^\top \phi( \tilde s_{t}') - {\bf v}_t^\top \phi( \tilde s_{t})
\end{align}

as an estimate for the TD error, where ${\bf v}_t$ corresponds to the value function parameter at time $t$.
$\phi( \tilde s_{t})$ corresponds to a feature vector of state $\tilde s_t$, sampled from RB $i$. 

From now on, unless explicitly mentioned, we shall consider $\delta_{t; i}$ to be defined according to Equation (\ref{eq:delta_linear}). Let $\bar V^{\pi_\theta} (s)$ denote the quantity

\begin{equation}
\label{eq:bar_V2}
    \bar V^{\pi_\theta} (s) = \sum_a \pi(a|s) \big( r(s, a) - \eta_{\theta} + \sum_{s' \in \mathcal{S}} P (s' | s, a)  {\bf v}^{\pi \top} \phi(s') \big)
\end{equation}

where ${\bf v}^{\pi \top} \phi(s')$ is an estimate of the value function $V^\pi (s')$ that is obtained upon convergence of a TD recursion (above) viz., $\lim_{t \rightarrow \infty} {\bf v}_t = {\bf v}^\pi$ with probability one. Also, let $\delta^\pi_{t; i}$ denote the associated quantity 

\[\delta^\pi_{t; i} = \tilde r_{t} - \eta_t + {\bf v}^{\pi \top} \phi( \tilde s_{t}') - {\bf v}^{\pi \top} \phi( \tilde s_{t}) \]
Then $\delta^\pi_{t; i}$ corresponds to a stationary estimate of the
TD error (with function approximation) under policy $\pi$. We have the following analog of Theorem
1 of \cite{sutton2000policy} and Lemma 4 of \cite{bhatnagar2008incremental}.

\begin{lemma}
\label{lemma:delta_psi2}
Let $e^{\pi_\theta} = \mathbb{E}_{s \sim \mu_\theta} \left[ \nabla \bar V^{\pi_\theta} (s) - \nabla {\bf v}^{\pi \top} \phi(s) \right] $
\begin{align*}
    & \mathbb{E} [\delta^\pi_{t; i} \psi(\tilde s_t, \tilde a_t) | \boldsymbol{\theta}] = \nabla \eta_{\boldsymbol\theta} + e^{\pi_\theta}
    %& - \mathbb{E}_{s \sim \mu^{\pi_\theta, a \sim \pi_\theta}} \big[ \nabla \log \pi_\theta (a|s) {\bf v}^{\pi \top} \phi(s) \big]
\end{align*}
\end{lemma}
\subsection{other lemmas}
We first prove the following lemmas:
\begin{lemma}
\label{lemma:expected_V_i2}
\[\mathbb{E}_{i \sim \boldsymbol{\beta}}[V^{\pi_\theta} (s; i)] = V^{\pi_\theta} (s)\]
\end{lemma}

\begin{proof}
According to equations (\ref{eq:V_i2}) (\ref{eq:Q_i2}):
\begin{align*}
    & \mathbb{E}_{i \sim \boldsymbol{\beta}}[V^{\pi_\theta} (s; i)] = \sum_{i} \beta_i \sum_{a} \pi_\theta(a|s) Q^{\pi_\theta} (s,a; i) \\
    & = \sum_{a} \pi_\theta(a|s) \sum_{i} \beta_i \big( r(s,a) - \eta(\boldsymbol{\theta}) \\
    & + \sum_{s'} P_i(s'|s,a) V^{\pi_\theta} (s')\big)\\
    & = \sum_{a} \pi_\theta(a|s) \big( r(s,a) - \eta(\boldsymbol{\theta}) + \sum_{s'} \sum_{i} \beta_i P_i(s'|s,a) V^{\pi_\theta} (s')\big)\\
    & = \sum_{a} \pi_\theta(a|s) \big( r(s,a) - \eta(\boldsymbol{\theta}) + \sum_{s'} P(s'|s,a) V^{\pi_\theta} (s')\big)\\
    & = \sum_{a} \pi_\theta(a|s) Q^{\pi_\theta} (s, a) = V^{\pi_\theta} (s)
\end{align*}
where the second to last equation is according to the definition in XXX. %(\ref{eq:Q_def}).
\end{proof}


\begin{lemma}
\label{lemma:Q_expec2}
\[(a) \mathbb{E}_{i \sim \boldsymbol{\beta}} [Q^{\pi_\theta} (s,a; i) \psi(s,a)] = Q^{\pi_\theta} (s,a) \psi(s,a)\]
\[(b) \mathbb{E}_{i \sim \boldsymbol{\beta}} [\hat Q^{\pi_\theta}_{\bf w} (s,a) \psi(s,a)] = \hat Q^{\pi_\theta}_{\bf w} (s,a) \psi(s,a)\]

\end{lemma}

\begin{proof}[Proof of lemma \ref{lemma:Q_expec2}]
For (a), according to $Q^{\pi_\theta} (s,a; i)$ definition in (\ref{eq:Q_i2}):
\begin{align*}
    & \mathbb{E}_{i \sim \boldsymbol{\beta}} [Q^{\pi_\theta} (s,a; i) \psi(s,a)] = \sum_{i=1}^K \beta_i Q^{\pi_\theta} (s,a; i)  \psi(s,a)\\
& = \sum_{i=1}^K \beta_i \big( r(s,a) - \eta_\theta  + \sum_{s'}P_i(s'|s,a) V^{\pi_\theta} (s)   \big) \psi(s,a) \\
& = \big( r(s,a) - \eta_\theta +   \sum_{s'} \sum_{i=1}^K \beta_i P_i(s'|s,a) V^{\pi_\theta} (s) \big) \psi(s,a)\\
& = \big( r(s,a) - \eta_\theta +   \sum_{s'} P(s'|s,a) V^{\pi_\theta} (s') \big) \psi(s,a) \\
& = Q^{\pi_\theta} (s,a) \psi(s,a)
\end{align*}

For (b), recall that $\hat Q^{\pi_\theta}_{\bf w} (s,a) = {\bf w}^\top \psi(s,a)$. Then:
\begin{align*}
    & \mathbb{E}_{i \sim \boldsymbol{\beta}} [\hat Q^{\pi_\theta}_{\bf w} (s,a) \psi(s,a)] = \mathbb{E}_{i \sim \boldsymbol{\beta}} [\psi(s,a)  \psi(s,a)^\top {\bf w}]\\
    & = \sum_{i=1}^K \beta_i \psi(s,a)  \psi(s,a)^\top {\bf w} = \psi(s,a)  \psi(s,a)^\top {\bf w} \\
& = \hat Q^{\pi_\theta}_{\bf w} (s,a) \psi(s,a)  
\end{align*}
since $\psi(s,a)$ are independent of $i$. 
\end{proof}




We next show that $\hat \nabla_{{\bf w}} \mathcal{E}^{\pi_\theta}_{\text{s2r}} ({\bf w})$ is an unbiased estimate for the real gradient $\nabla_{{\bf w}} \mathcal{E}^{\pi_\theta}_{\text{s2r}} ({\bf w})$.
\begin{lemma}
\label{lemma:unbiased_critic_gradient}
\[ \mathbb{E} \big[ \hat \nabla_{{\bf w}} \mathcal{E}^{\pi_\theta}_{\text{s2r}} ({\bf w})\big] = \nabla_{{\bf w}} \mathcal{E}^{\pi_\theta}_{\text{s2r}} ({\bf w}) \]
\end{lemma}

\begin{proof}[Proof of Lemma \ref{lemma:unbiased_critic_gradient}]
Recall that our probability measure contains the state stationary distribution, the policy and the random "coin" $\boldsymbol{\beta}$. In addition, recall that $\nabla_{{\bf w}} \hat{Q}^{\pi_\theta}_{{\bf w}}(s,a) = \psi(s,a)$.
\begin{align*}
    & \mathbb{E}_{s \sim \mu^{\pi_\theta}, a \sim \pi_{\theta}, i \sim \boldsymbol{\beta}} \big[ \hat \nabla_{{\bf w}} \mathcal{E}^{\pi_\theta}_{\text{s2r}} ({\bf w})\big] \\
    & = \mathbb{E}_{s \sim \mu^{\pi_\theta}, a \sim \pi_{\theta}, i \sim \boldsymbol{\beta}} \big[  - \big( Q^{\pi_\theta} (s,a; i) - \hat{Q}^{\pi_\theta}_{{\bf w}}(s,a) \big) \nabla_{{\bf w}} \hat{Q}^{\pi_\theta}_{{\bf w}}(s,a) \big] \\
    & = \mathbb{E}_{s \sim \mu^{\pi_\theta}, a \sim \pi_{\theta}} \big[ \mathbb{E}_{i \sim \boldsymbol{\beta}} [ - \big( Q^{\pi_\theta} (s,a; i)  - \hat{Q}^{\pi_\theta}_{{\bf w}}(s,a) \big) \psi(s,a)]  \big] \\
    & = \mathbb{E}_{s \sim \mu^{\pi_\theta}, a \sim \pi_{\theta}} \big[ - \big( Q^{\pi_\theta} (s,a) - \hat{Q}^{\pi_\theta}_{{\bf w}}(s,a) \big) \nabla_{{\bf w}} \hat{Q}^{\pi_\theta}_{{\bf w}}(s,a) \big] \\
    & = \nabla_{{\bf w}} \mathcal{E}^{\pi_\theta}_{\text{s2r}} ({\bf w})
\end{align*}
where we used Lemma \ref{lemma:Q_expec2}.
\end{proof}


\subsection{Proof of Lemma \ref{lemma:unbiased_delta} }
\begin{proof}[Proof of Lemma \ref{lemma:unbiased_delta}]
The proof is based on Lemma 3 in \cite{bhatnagar2009natural}. Recall that when taking an expectation, we relate our probability measure that includes the transition probabilities defined in MDP $i$, $P_i$, the stochastic policy $\pi_\theta$ and the probability distribution $\boldsymbol{\beta}$ that selects which MDP we sample the selected transition $\tilde{\mathcal{O}}_{t;i}$. 

By the definition of the TD-error in (\ref{eq:delta_def4}): 
\begin{align*}
    & \mathbb{E} \left[\delta_{t; i} | \tilde s_{t}, \tilde a_{t}, \pi_\theta \right] = \mathbb{E} \left[ \tilde r_{t} - \eta_{t} + \hat{V} ( \tilde s_{t}' ) - \hat{V} ( \tilde s_{t}) \middle| \tilde s_{t}, \tilde a_{t}, \pi_\theta \right] \\
    & \mathbb{E}_{i \sim \boldsymbol\beta, \cdot \sim \frac{1}{N} \tilde s'_t \sim P_i(\cdot|\tilde s_t, \tilde a_t)} \left[\delta_{t; i} | \tilde s_{t}, \tilde a_{t}, \pi_\theta \right] \\
    & = r( \tilde s_{t}, \tilde a_{t}) - \eta_{\boldsymbol\theta} + \mathbb{E} \left[ \hat{V} ( \tilde s_{t}' )  - \hat{V} ( \tilde s_{t} ) \middle| \tilde s_{t}, \tilde a_{t}, \pi \right]
\end{align*}
where the last equality follows the unbiased assumption for $\eta_t$ and the definition of the expected reward $r(s,a)$. Next, we use the unbiased assumption for the estimator $ \hat{V} ( \tilde s_{t} )$, given 
$\tilde s_{t}, \tilde a_{t}$ and $\pi_\theta$:
\begin{align*}
    & \mathbb{E} \left[ \hat{V} ( \tilde s_{t} ) \middle| \tilde s_{t}, \tilde a_{t}, \pi_\theta \right] = V^{\pi_\theta} ( \tilde s_{t}  )
\end{align*}
Let's look at the following term:
\begin{align*}
    & \mathbb{E} \left[ \hat{V} (\tilde s_{t}') \middle| \tilde s_{t}, \tilde a_{t}, \pi_\theta \right] = \mathbb{E} \left[ \mathbb{E} \left[\hat{V} (\tilde s_{t}') \middle| \tilde s'_{t}, \pi_\theta \right] \middle| \tilde s_{t}, \tilde a_{t}  \right]\\
    & = \mathbb{E} \left[ V^{\pi_\theta} (\tilde s_{t}')  \middle| \tilde s_{t}, \tilde a_{t}  \right] = \mathbb{E}_{i \sim \boldsymbol{\beta}, \tilde s_t' \sim P_i} \left[ V^{\pi_\theta} ( \tilde s_{t}') \middle| \tilde s_{t}, \tilde a_{t} \right] \\
    & = \sum_{\tilde s_{t}' \in \mathcal{S}} \sum_{i=1}^K \beta_i P_i (\tilde s_{t}' | \tilde s_{t}, \tilde a_{t}) V^{\pi_\theta} ( \tilde s_{t}' ) \\
    & = \sum_{\tilde s_{t}' \in \mathcal{S}} P(\tilde s_{t}' | \tilde s_{t}, \tilde a_{t}) V^{\pi_\theta} ( \tilde s_{t}' )
\end{align*}
In addition:
\[
r(\tilde s_{t}, \tilde a_{t}) - \eta_{\boldsymbol{\theta}} + \sum_{\tilde s_{t}' \in \mathcal{S}} P (\tilde s_{t}' | \tilde s_{t}, \tilde a_{t}) V^{\pi_\theta} ( \tilde s_{t}' ) = Q^{\pi_\theta} (\tilde s_{t} , \tilde a_{t}) \]
Then:
\[\mathbb{E}[\delta_{t; i} | \tilde s_{t}, \tilde a_{t}, \pi_\theta] =  Q^{\pi_\theta} (\tilde s_{t} , \tilde a_{t}) - V^{\pi_\theta}  ( \tilde s_{t}) = A^{\pi_\theta} (\tilde s_{t} , \tilde a_{t})\]
\end{proof}

\subsection{Proof of Lemma \ref{lemma:delta_psi2}}

\begin{proof}[Proof of Lemma \ref{lemma:delta_psi2}]
The proof is based on Lemma 4 in \cite{bhatnagar2009natural}. We refer here to the same probability measure as mentioned in the proof for Lemma \ref{lemma:unbiased_delta}. 
By the definition of the TD-error in (\ref{eq:delta_def4}): 
\begin{align*}
    & \mathbb{E} [\delta^\pi_{t; i} \psi(\tilde s_t, \tilde a_t) | \boldsymbol{\theta}] = \mathbb{E} \big [ \mathbb{E}_{i \sim \beta, \tilde s' \sim P_i} [\delta^\pi_{t; i} | \tilde s_t, \tilde a_t] \psi(\tilde s_t, \tilde a_t) | \boldsymbol{\theta}  \big] \\
    & = \mathbb{E}_{s \sim \mu_\theta, a \sim \pi_{\theta}} \big [  r(s,a) - \eta_{\boldsymbol\theta} \\
    & + \sum_{s'} \sum_{i} \beta_i P_i(s'|s,a) {\bf v}^{\pi \top} \phi(s') - {\bf v}^{\pi \top} \phi(s)\big) | s, a] \psi(s, a) | \boldsymbol{\theta}  \big] \\
    & = \mathbb{E}_{s \sim \mu_\theta, a \sim \pi_{\theta}} \big[ \nabla \log \pi_\theta (s|a) \big( r(s,a) - \eta_{\boldsymbol\theta} \\
    & + \sum_{s'} P(s'|s,a) {\bf v}^{\pi \top} \phi(s') - {\bf v}^{\pi \top} \phi(s)\big) \big]
\end{align*}

The rest of the proof follows the same as in the proof of Lemma 4 in \cite{bhatnagar2009natural}. 

\iffalse
Now, from (\ref{eq:bar_V2}):
\begin{align*}
    & \nabla \bar V^{\pi_\theta} (s) = \sum_a \nabla \pi(a|s) \big( r(s, a) - J(\pi) \\
    & + \sum_{s' \in \mathcal{S}} {\bf P} (s' | s, a)  {\bf v}^{\pi \top} \phi(s') \big) \\
    & + \sum_a \pi(a|s) \big( - \nabla J(\pi) + \sum_{s' \in \mathcal{S}} {\bf P} (s' | s, a)  \nabla {\bf v}^{\pi \top} \phi(s') \big)
\end{align*}

Then:
\begin{align*}
    & \mathbb{E}_{s \sim \mu^{\pi_\theta}} [\nabla \bar V^{\pi_\theta} (s)] = \mathbb{E}_{s \sim \mu^{\pi_\theta}} \big[ \sum_a \nabla \pi(a|s) \big( r(s, a) - J(\pi) \\
    & + \sum_{s' \in \mathcal{S}} {\bf P} (s' | s, a)  {\bf v}^{\pi \top} \phi(s') \big) \\
    & + \sum_a \pi(a|s) \big( - \nabla J(\pi) + \sum_{s' \in \mathcal{S}} {\bf P} (s' | s, a)  \nabla {\bf v}^{\pi \top} \phi(s') \big) \big] \\
    & = \mathbb{E}_{s \sim \mu^{\pi_\theta}, a \sim \pi_\theta} \big[ \nabla \log \pi_\theta (a|s) \big( r(s, a) - J(\pi) \\
    & + \sum_{s' \in \mathcal{S}} {\bf P} (s' | s, a)  {\bf v}^{\pi \top} \phi(s') \big) \\
    &  - \nabla J(\pi) + \sum_{s' \in \mathcal{S}} {\bf P} (s' | s, a)  \nabla {\bf v}^{\pi \top} \phi(s') \big) \big] \\
    & = \mathbb{E} [\delta^\pi_{t; i} \psi(s_t, a_t) | \boldsymbol{\theta}] + \mathbb{E}_{s \sim \mu^{\pi_\theta}, a \sim \pi_\theta} \big[ \nabla \log \pi_\theta (a|s) {\bf v}^{\pi \top} \phi(s) \big] \\
    & - \mathbb{E}_{s \sim \mu^{\pi_\theta}, a \sim \pi_\theta} \big[ 
     \nabla J(\pi) - \sum_{s' \in \mathcal{S}} {\bf P} (s' | s, a)  \nabla {\bf v}^{\pi \top} \phi(s') \big) \big] \\
     & = \mathbb{E} [\delta^\pi_{t; i} \psi(s_t, a_t) | \boldsymbol{\theta}] + \mathbb{E}_{s \sim \mu^{\pi_\theta, a \sim \pi_\theta}} \big[ \nabla \log \pi_\theta (a|s) {\bf v}^{\pi \top} \phi(s) \big] \\
    & - \nabla J(\pi) + \mathbb{E}_{s \sim \mu^{\pi_\theta}, a \sim \pi_\theta} \big[ 
      \sum_{s' \in \mathcal{S}} {\bf P} (s' | s, a)  \nabla {\bf v}^{\pi \top} \phi(s')  \big] \\
\end{align*}
Now observe that $\mu^{\pi_\theta} (s)$ correspond to the stationary probabilities that satisfy
\begin{equation}
\label{eq:mu2}
    \mu^{\pi_\theta} (s) = \sum_{s'' \in \mathcal{S}} \mu^{\pi_\theta} (s'') p^\pi (s'', s), s \in \mathcal{S}
\end{equation}
 with $\sum_{s'' \in \mathcal{S}} \mu^{\pi_\theta} (s'') = 1$.
where $p^\pi (s'', s) = \sum_{a \in \mathcal{A}} \pi(a | s'') {\bf P} (s | s'', a) $ are the transition probabilities of the resulting Markov chain under policy $\pi$. Hence
\begin{align*}
    & \mathbb{E}_{s \sim \mu^{\pi_\theta}, a \sim \pi_\theta} \big[ 
      \sum_{s' \in \mathcal{S}} {\bf P} (s' | s, a)  \nabla {\bf v}^{\pi \top} \phi(s') \big] \\
      & = \mathbb{E}_{s \sim \mu^{\pi_\theta}, s' \sim p^{\pi} (s,s')} \big[ 
       \nabla {\bf v}^{\pi \top} \phi(s') \big] \\
       & = \sum_{s \in \mathcal{S}} \sum_{s' \in \mathcal{S}} \mu^{\pi_\theta}(s) p^{\pi} (s, s')  \nabla {\bf v}^{\pi \top} \phi(s') \\
       & = \sum_{s' \in \mathcal{S}} \mu^{\pi_\theta}(s') \nabla {\bf v}^{\pi \top} \phi(s') \\
       & = \sum_{s \in \mathcal{S}} \mu^{\pi_\theta}(s) \nabla {\bf v}^{\pi \top} \phi(s)
\end{align*}

Then:
\begin{align*}
    & \mathbb{E} [\delta^\pi_{t; i} \psi(s_t, a_t) | \boldsymbol{\theta}] = \nabla J(\pi) \\
    & + \mathbb{E}_{s \sim \mu^{\pi_\theta}} \big[ \nabla \bar V^{\pi_\theta} (s) - \nabla {\bf v}^{\pi \top} \phi(s) \big] \\
    & - \mathbb{E}_{s \sim \mu^{\pi_\theta, a \sim \pi_\theta}} \big[ \nabla \log \pi_\theta (a|s) {\bf v}^{\pi \top} \phi(s) \big]
\end{align*}

\fi

\end{proof}



\subsection{Lemmas for bounding distances between eigenvalues of Markov Processes}
Before we proceed with the technical proofs, we introduce some notations that will help us in the following Lemmas.

Let $\{X_t\}_{t \ge 0}$ be a Markov process with transition probability function ${\bf P}_X$. Let $\lambda_1^X, \ldots, \lambda_{|\mathcal{S}|}^X$ be the eigenvalues of ${\bf P}_X$, ordered by $|\lambda_1^X| \ge \ldots |\lambda_{|\mathcal{S}|}^X|$. 

The matrix ${\bf P}_X$ is a stochastic, hence $\lambda_1^X = 1$. Denote the second largest eigenvalue of ${\bf P}_X$ by $\lambda^X_2$, where $|\lambda^X_2| < 1$.  

Let $\bar{D}\Big(\lambda_i^X, \epsilon \Big)$
be the closed disk with radius $\epsilon$ and center $\lambda_i^X$. 

We will use the same notations also for these stochastic processes:
$\{Y_t\}_{t \ge 0}$, $\{W_t\}_{t \ge 0}$, $\{Z_t\}_{t \ge 0}$ and $\{U_t\}_{t \ge 0}$. 

Note: Later we will use these notations as follows:
\begin{itemize}
    \item $\{X_t\}_{t \ge 0}$ - Real Markov Process.
    \item $\{Y_t\}_{t \ge 0}$ - Sim Markov Process.
    \item $\{W_t\}_{t \ge 0}$ - Slow real Markov Process (by factor $p$).
    \item $\{Z_t\}_{t \ge 0}$ - Real+Sim Markov Process (by interpolation with $\beta$).
    \item $\{U_t\}_{t \ge 0}$ - slow Real + fast Sim Markov Process (by interpolation with $\beta$).
\end{itemize}

\begin{lemma}[Continuity of Eigenvalues. Corollary VI.1.6 in \cite{bhatia2013matrix}]
\label{lemma:beta_continuity}
Let $\beta \rightarrow {\bf P}(\beta)$ be a continuous map from an interval I into the space of $|\mathcal{S}| \times |\mathcal{S}|$ matrices. Then, there exist continuous functions $\lambda_1(\beta), \lambda_2(\beta), \ldots \lambda_{|\mathcal{S}|}(\beta)$ that, for each $\beta \in I$, are the eigenvalues of ${\bf P}(\beta)$.

\end{lemma}

\begin{lemma}[Eigenvalues do not deviate much for perturbed matrices. Theorem VI.5.1 in \cite{bhatia2013matrix}]
\label{lemma:pertub_bound}
Let ${\bf P}_X$ be a normal matrix and let ${\bf P}_Y$ be any matrix such that
\[\| {\bf P}_X - {\bf P}_Y\| = \epsilon_0\]
and
\[\epsilon_0 < \frac{1}{2} \min_{i, j \neq i} |\lambda_{i}^X - \lambda_{j}^X|\]
where $\lambda_{i}^X$ and $\lambda_{j}^X$ are distinct eigenvalue of ${\bf P}_X$. 
Let
\[d(\sigma({\bf P}_X), \sigma({\bf P}_Y)) = \min_{\sigma} \max_{1 \le j \le |\mathcal{S}|} |\lambda^X_j - \lambda^Y_{\sigma(j)}|\]
and $\sigma({\bf P}_X)$ is an unordered $|\mathcal{S}|$-tuple whose entries are the eigenvalues of ${\bf P}_X$.  
Then:
\[d(\sigma({\bf P}_X), \sigma({\bf P}_Y))\le \| {\bf P}_X - {\bf P}_Y\|\]
*** Corollary VI.6.4 in \cite{bhatia2013matrix} says this bound on every norm with p-norm $p\ge 2$ and if ${\bf P}_Y$ is also normal.
\end{lemma}



\begin{lemma}[Slowing process by factor $p$]
\label{lemma:unfair_coin}
Let $\{X_t\}_{t \ge 0}$ be a Markov process. Let B be a Bernoulli random variable with distribution:
\[\mathbb{P}(B=1)=p\]
\[\mathbb{P}(B=0)=1 - p\]
where $0 \le p \le 1$. Let $\{W_t\}_{t \ge 0}$ be a stochastic process which satisfies:
\begin{align*}
    W_{t+1} = \begin{cases}
    X_{t+1} & \text{if } B=1 \\
    W_t & \text{if } B=0 
    \end{cases}
\end{align*}
where $X_{t+1} \sim {\bf P}_X(X_{t+1}|W_t)$. Then:
\begin{enumerate}
    \item $\{W_t\}_{t \ge 0}$ is a Markov process.
    \item If $p=0$, then $\lambda^W_2=1$, if $0 < p \le 1$
    \[|\lambda^X_2| < |\lambda^W_2| = p \cdot |\lambda^X_2| + 1-p < 1\]
\end{enumerate}
\end{lemma}

\begin{proof}[Proof of Lemma \ref{lemma:unfair_coin}]
We can write ${\bf P}_W$ explicitly:
\begin{equation}
\label{eq:Pw}
    {\bf P}_W = p \cdot {\bf P}_{X} + (1-p) {\bf I}
\end{equation}
where ${\bf I}$ is the identity matrix with size $|\mathcal{S}| \times |\mathcal{S}|$. Since ${\bf P}_{X}$ is Markovian, it only depends on the last state, implying that also ${\bf P}_{W}$ depends only on the last state, making it a Markovian process. 

We are interested in finding $\lambda^W_2$, the second largest eigenvalue of ${\bf P}_{W}$. Note that since ${\bf P}_{X}$ is a stochastic matrix, then by Equation \ref{eq:Pw}, ${\bf P}_{W}$ is also a stochastic matrix, hence its first eigenvalue equals to 1. Let ${\bf v}_X$ be the eigenvector which corresponds to $\lambda^X_2$. Then:
\[{\bf P}_{X} {\bf v}_X = \lambda^X_2 {\bf v}_X\]

Now we compute the following:
\begin{align*}
    {\bf P}_{W} {\bf v}_X & = \Big( p \cdot {\bf P}_{X} + (1-p) {\bf I} \Big) {\bf v}_X \\
     & = p \cdot {\bf P}_{X}{\bf v}_X + (1-p) {\bf v}_X \\
     & = p \cdot \lambda^X_2 {\bf v}_X + (1-p) {\bf v}_X \\
     & = \big( p \cdot \lambda^X_2 + (1-p) \big) {\bf v}_X \\
     & = \tilde{\lambda} {\bf v}_X 
\end{align*}
Then, $\tilde{\lambda} = p \cdot \lambda^X_2 + (1-p)$ is an eigenvalue of ${\bf P}_{W}$ corresponding to the eigenvector ${\bf v}_X$. 


If $p=0$, then $\tilde{\lambda} = 1$. If $0 < p \le 1$, $\tilde{\lambda} < 1$.

In addition, $\tilde{\lambda}$ satisfies:
\[|\tilde{\lambda}| \le |\lambda^W_2|\]
\[\Rightarrow |\lambda^W_2| \ge |p \cdot \lambda^X_2 + (1-p)| = p |\lambda^X_2| + 1-p\]
\[\Rightarrow |\lambda^X_2| \le |\lambda^W_2| < 1\]

\end{proof}


\begin{lemma}[Mixing two Markovian processes]
\label{lemma:mixing_process}
Let B be a Bernoulli random variable with distribution:
\[P(B=1)=\beta\]
\[P(B=0)=1 - \beta\]

where $0\le \beta \le 1$.

Let $\{X_t\}_{t \ge 0}$ and $\{Y_t\}_{t \ge 0}$ be two Markov processes satisfying:
\[\| {\bf P}_X - {\bf P}_Y\| = \epsilon\]



Let $\{Z_t\}_{t \ge 0}$ be a mixing of these process according to the random Bernoulli variable B, such that when B=1, $Z_t=X_t$ and when $B=0$ $Z_t=Y_t$. Then:
\begin{enumerate}
    \item $\{Z_t\}_{t \ge 0}$ is a Markov process. 
    \item Let
    \[\epsilon_1 < \frac{1}{2} \min_{i, j \neq i} |\lambda_{i}^Y - \lambda_{j}^Y|\] 
    where $\lambda_{i}^Y$ and $\lambda_{j}^Y$ are distinct eigenvalue of ${\bf P}_Y$. If ${\bf P}_Y$ is normal matrix and if $\epsilon \le \epsilon_1$, then:
    \[d(\sigma({\bf P}_Y), \sigma\big( {\bf P}_Z(\beta) \big)\le \beta \epsilon_1 \]
    %\[|\lambda^Y_2 - \lambda^Z_2(\beta)| \le \beta \epsilon_1\]
\end{enumerate}
\end{lemma}

\begin{proof}[Proof of Lemma \ref{lemma:mixing_process}]
Observe that we can write ${\bf P}_Z$ as a function of $\beta$:
\[{\bf P}_Z (\beta) = \beta {\bf P}_X + (1-\beta) {\bf P}_Y\]

The process $\{Z_t\}_{t \ge 0}$ depends only on the last state, since its transition probability matrix ${\bf P}_Z$ depends only on ${\bf P}_X$ and ${\bf P}_Y$, which are matrices of Markov Processes. Hence, $\{Z_t\}_{t \ge 0}$ is also a Markov process.

For the second part of the proof, we will use the proof of Theorem VI.5.1 in \cite{bhatia2013matrix}).
${\bf P}_Z (\beta)$ is a continuous map from $[0,1]$ to the space of $|\mathcal{S}| \times |\mathcal{S}|$ matrices. We have that ${\bf P}_Z (0) = {\bf P}_Y$, ${\bf P}_Z (1) = {\bf P}_X$. Note that $\| {\bf P}_Y - {\bf P}_Z (\beta) \| = \beta \epsilon$ and so all the eigenvalues of ${\bf P}_Z (\beta) $ also lie in the disks $\bar{D}\Big(\lambda^i_Y, \epsilon \Big)$ for each $0 \le \beta \le 1$. By Lemma \ref{lemma:beta_continuity}, as $\beta$ moves from 0 to 1, the eigenvalues of ${\bf P}_Z (\beta)$ trace continuous curves that join the eigenvalues of ${\bf P}_X$ to those of ${\bf P}_Y$. None of these curves can jump from one of the disks to another. 

If ${\bf P}_Y$ is normal matrix, then, by Lemma \ref{lemma:pertub_bound}:
\[d(\sigma({\bf P}_Y), \sigma({\bf P}_Z(\beta)))\le \| {\bf P}_Y - {\bf P}_Z (\beta)\| = \beta \epsilon \le \beta \epsilon_1\]
%By similar arguments we provided in of Lemma \ref{lemma:pertub_bound}, we have:
%\[|\lambda^Y_2 - \lambda^Z_2(\beta)| \le \beta \epsilon_1\]
\end{proof}

\begin{lemma}
\label{lemma:bound_norm_slow}
Let $\{X_t\}_{t \ge 0}$ and $\{Y_t\}_{t \ge 0}$ be two Markov processes, satisfying:
\[\| {\bf P}_X - {\bf P}_Y\| = \epsilon\]
Let
$\{W_t\}_{t \ge 0}$ be a stochastic process such that
\[{\bf P}_W = p \cdot {\bf P}_X + (1-p) {\bf I}\]
Then:
\[ \| {\bf P}_W - {\bf P}_Y\| \le p \cdot \epsilon + (1-p) \| {\bf I} - {\bf P}_Y\| \]
\end{lemma}

\begin{proof}[Proof of Lemma \ref{lemma:bound_norm_slow}]
\begin{align*}
    \| {\bf P}_W - {\bf P}_Y\| & =  \| p \cdot {\bf P}_X + (1-p) {\bf I} - {\bf P}_Y\|\\
    & = \| p \cdot {\bf P}_X + (1-p) {\bf I} - p \cdot {\bf P}_Y - (1-p) {\bf P}_Y\| \\
    & = \| p \cdot \big( {\bf P}_X - {\bf P}_Y \big) + (1-p)  \big( {\bf I} - {\bf P}_Y \big)\|\\
    & \le p \| {\bf P}_X - {\bf P}_Y \| + (1-p)  \| {\bf I} - {\bf P}_Y \|\\
    & =  p \cdot \epsilon + (1-p)  \| {\bf I} - {\bf P}_Y \|
\end{align*}

\end{proof}

\begin{lemma}[Mixing Slow Markov Process with fast Perturbed Markov Process]
\label{lemma:mixing_slow_fast}
Let $\{X_t\}_{t \ge 0}$ be a Markov process. Let $\{W_t\}_{t \ge 0}$ be a of slowing $\{X_t\}_{t \ge 0}$ by a factor $p$ as described in Lemma \ref{lemma:unfair_coin}.

Let $\{Y_t\}_{t \ge 0}$ be a perturbed Markov process of $\{X_t\}_{t \ge 0}$, such that:
\[\| {\bf P}_X - {\bf P}_Y\| = \epsilon\]

Let  $\{U_t\}_{t \ge 0}$ be a process of mixing $\{W_t\}_{t \ge 0}$ and $\{Y_t\}_{t \ge 0}$ with interpolation coefficient $\beta$, as described in Lemma \ref{lemma:mixing_process}.
Then:
\begin{enumerate}
    \item $\{U_t\}_{t \ge 0}$ is a Markov Process.
    \item Let
    \[\epsilon_1 < \frac{1}{2} \min_{i, j \neq i} |\lambda_{i}^Y - \lambda_{j}^Y|\] 
    where $\lambda_{i}^Y$ and $\lambda_{j}^Y$ are distinct eigenvalue of ${\bf P}_Y$. If ${\bf P}_Y$ is normal matrix and if $\big(p \cdot \epsilon + (1-p) \| {\bf I} - {\bf P}_Y\|  \big) \le \epsilon_1$, then:
    \[d \Big(\sigma({\bf P}_Y), \sigma\big( {\bf P}_U(\beta) \big) \Big)\le \beta \epsilon_1\]
    %\[|\lambda^Y_2 - \lambda^U_2(\beta)| \le \beta \epsilon_1\]
    \item Let
    \[\epsilon_0 < \frac{1}{2} \min_{i,j \neq i} |\lambda_{i}^X - \lambda_{j}^X|\] 
    where $\lambda_{i}^X$ and $\lambda_{i}^X$ are distinct eigenvalue of ${\bf P}_X$. If ${\bf P}_X$ and ${\bf P}_Y$ are normal matrices and if $\epsilon \le \epsilon_0$ and $\big(p \cdot \epsilon + (1-p) \| {\bf I} - {\bf P}_Y\|  \big) \le \epsilon_1$ , then:
    \[d \Big(\sigma({\bf P}_X), \sigma\big( {\bf P}_U(\beta) \big) \Big)\le \epsilon_0 + \beta \epsilon_1\]
    %\[|\lambda^X_2 - \lambda^U_2(\beta)| \le \epsilon_0 + \beta \epsilon_1\]
\end{enumerate}
\end{lemma}

\begin{proof}[Proof of Lemma \ref{lemma:mixing_slow_fast}]

{\bf Proof of (1.):} We recall that according to Lemma \ref{lemma:unfair_coin},
 $\{W_t\}_{t \ge 0}$ is a Markov process that is a "slow" version on $\{X_t\}_{t \ge 0}$, satisfying:
 \[{\bf P}_W = p \cdot {\bf P}_X + (1-p){\bf I} \]

$\{U_t\}_{t \ge 0}$ is a process of mixing $\{W_t\}_{t \ge 0}$ and $\{Y_t\}_{t \ge 0}$, thus, its transition probability ${\bf P}_U$ satisfies:

\[{\bf P}_U (\beta) = \beta {\bf P}_W + (1-\beta) {\bf P}_Y\]
The process $\{U_t\}_{t \ge 0}$ depends only on the last state, since its transition probability matrix ${\bf P}_U$ depends only on ${\bf P}_W$ and ${\bf P}_Y$, which are stochastic matrices of Markov Processes. Hence, $\{U_t\}_{t \ge 0}$ is also a Markov process.

{\bf Proof of (2.):} We are interested in bounding:
\begin{align*}
    \| {\bf P}_Y - {\bf P}_U (\beta)\| = \| {\bf P}_Y - \beta {\bf P}_W - (1-\beta) {\bf P}_Y\| = \beta \| {\bf P}_W - {\bf P}_Y\| \le \beta \big(p \cdot \epsilon + (1-p) \| {\bf I} - {\bf P}_Y\|  \big) 
\end{align*}
where the inequality is according to Lemma \ref{lemma:bound_norm_slow}.
Now that we have $\| {\bf P}_Y - {\bf P}_U (\beta)\|$ and we showed that both ${\bf P}_Y$ and ${\bf P}_U (\beta)$ are Markov processes, we can use the same arguments as in Lemma \ref{lemma:mixing_process} and conclude that if 
\[\big(p \cdot \epsilon + (1-p) \| {\bf I} - {\bf P}_Y\|  \big) \le \epsilon_1\]
then

\[d \Big(\sigma({\bf P}_Y), \sigma\big( {\bf P}_U(\beta) \big) \Big)\le \beta \epsilon_1\]

%\[|\lambda^Y_2 - \lambda^U_2(\beta)| \le \beta \epsilon_1 \]

{\bf Proof of (3.):} 
If $\epsilon \le \epsilon_0$, $p \cdot \epsilon + (1-p) \| {\bf I} - {\bf P}_Y\|   \le \epsilon_1$ and both ${\bf P}_X$ and ${\bf P}_Y$ are normal matrices, then: 

\begin{align*}
    d \Big(\sigma({\bf P}_X), \sigma\big( {\bf P}_U(\beta) \big) \Big) = XXXXX
\end{align*}

CONTINUE 

%\begin{align*}
%    |\lambda^X_2 - \lambda^U_2(\beta)| = |\lambda^X_2 - \lambda^Y_2 + \lambda^Y_2 - \lambda^U_2(\beta)| \le |\lambda^X_2 - \lambda^Y_2| + |\lambda^Y_2 - \lambda^U_2(\beta)| \le \epsilon_0 + \beta  \epsilon_1 
%\end{align*}
where the first inequality due to the triangle inequality and in the last inequality we used Lemma \ref{lemma:pertub_bound}.

\end{proof}

\subsection{Continuity of eigenvectors}
Let ${\bf x}$ be a left eigenvector of matrix ${\bf P} \in \mathbb{R}^{n \times n}$ corresponding to eigenvalue $\lambda$, then:
\[{\bf x}^\top {\bf P} = \lambda {\bf x}^\top\]
\[{\bf x}^\top ({\bf P} - \lambda {\bf I}) = {\bf 0}\]

Since ${\bf P}$ is a stochastic matrix, it has a left eigenvector $\boldsymbol{\mu}$ correspondig to eigenvalue $\lambda=1$, where $\boldsymbol{\mu}$ is the stationary distribution of ${\bf P}$, then:
\[\boldsymbol{\mu}^\top ({\bf P} - {\bf I}) = {\bf 0}\] 
From the rank-nullity theorem:
\[n = rank({\bf P - I}) + null({\bf P - I})\]
\[null({\bf P - I}) = dim\big(ker({\bf P - I}) \big)\]
\[dim\big(ker({\bf P - I}) \big) = \big| \{ {\bf y} \ | \ ({\bf P - I}){\bf y} = 0 \cdot {\bf y} = {\bf 0}\}\big|\]

The kernel of ${\bf P - I}$ is precisely the eigenspace corresponding to eigenvalue 0.  The matrix ${\bf P - I}$ has eigenvalue of 0 with multipicity 1, then 
\[dim\big(ker({\bf P - I}) \big) = 1\]
\[\Rightarrow rank({\bf P - I}) = n - 1\]
This means we have a linear system with $n-1$ equations.$ ({\bf P - I})$ is not invertible and there are infinite number of solutions. However, if we add the constraint of $\|\boldsymbol{\mu}\|=1$ (the stationary distribution is a vector of probabilities summing to 1), we add another equation to the system and now we have a single solution. Thus, we can view $\boldsymbol{\mu}$ as a function of ${\bf P}$ and $\lambda$ with only one image to each input. Since ${\bf P}$ is continuous in $\beta$
\[{\bf P} = \beta {\bf P}_1 + (1-\beta)  {\bf P}_2\]
and since $\lambda$ is continuous (XXXX Bahita), then $\boldsymbol{\mu}$ is a composition of continuous functions, thus it is continuous. 

ADD: ${\bf P}$ is irreducible and aperiodic. 

Note that the contiouty of$\boldsymbol{\mu}$ is over the unit circle, and it is not a straight line. 

Look at: CONVERGENCE THEOREM FOR FINITE MARKOV CHAINS ARI FREEDMAN. 

https://math.uchicago.edu/~may/REU2017/REUPapers/Freedman.pdf


See also: Course 214 Section 1: Basic Theorems of Complex Analysis Second Semester 2008 - Proposition 1.14. page 13. 

https://www.maths.tcd.ie/~dwilkins/Courses/214/214S1\_0708.pdf

\subsection{Convergance of replay buffer}
The Effects of Memory Replay in Reinforcement
Learning, 
Ruishan Liu, 2018, IEEE

\subsection{convergance proof}
proof sketch:
\begin{enumerate}
    \item formalize a replay buffer as a Markov chain + ergodic, irreducible
    \item state the probability distribution of sampling from a replay buffer
    \item state our algorithm of sampling from two replay buffers with different probabilities
    \item algorithm convergence - two time scale + Bounded Martingale difference
    \item state all the necessary assumptions. 
    \item Next - what is the point of convergance - we dont know it exactly, how ever it is close to the real point. why? Because we are avereging with the stationary distribution of sim+real. and it is continous, and close to the stationary distribution of real only. 
\end{enumerate}

Our aim is to show that the iterations of the actor and critic in our algorithm, that samples from teo replay buffers, and optimize with different proability measures, converge. For this, we will first need to prove the following steps: Sampling from a Replay buffer is a Markov process; This process is erodic, etc....; The iterations form an ode with bounded martingale difference. 
